# Supplementary material for: A Generic Framework for Conformal Fairness
Source: arXiv:2505.16115 source file (2025-10-20)
Supplement: Supplementary file 1 [file extra_batch_gcp.tex]

\begin{figure}[ht!]
    \centering
    \begin{subfigure}{0.5\textwidth}
        \includegraphics[width=\linewidth]{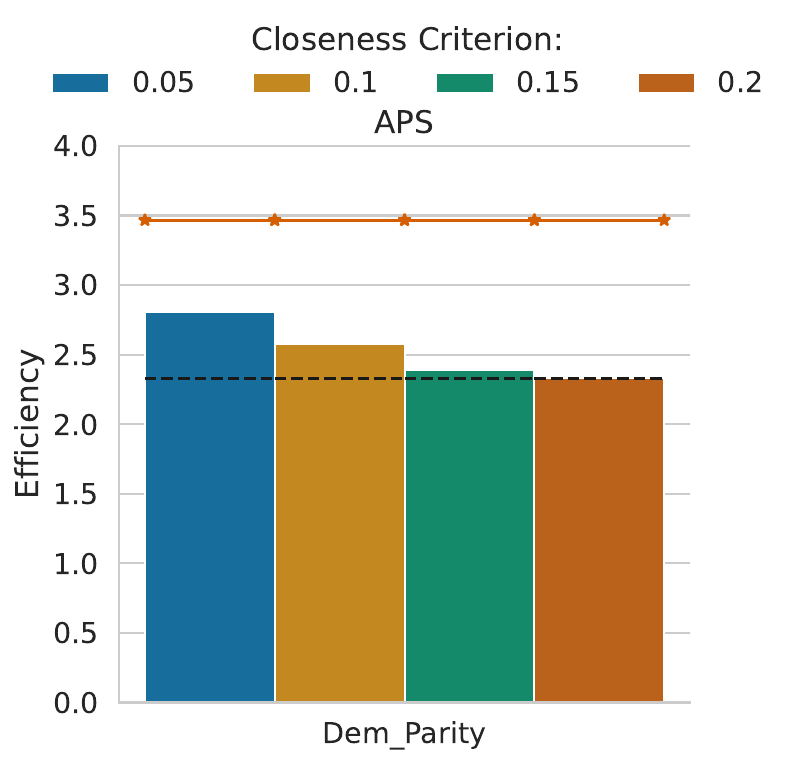}
    \end{subfigure}%
    \begin{subfigure}{0.5\textwidth}
        \includegraphics[width=\linewidth]{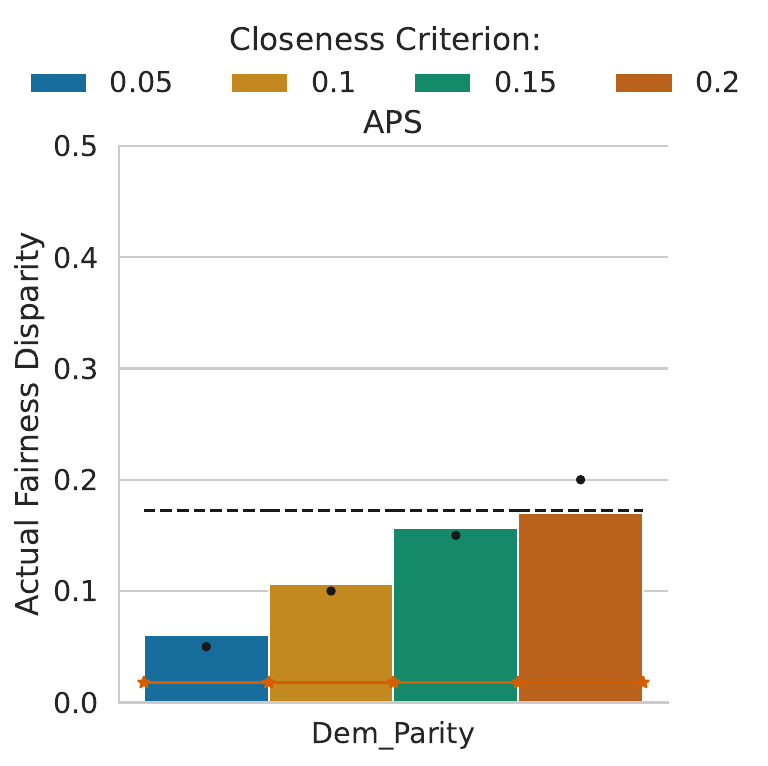}
    \end{subfigure}
    \caption{\small\textbf{Credit.} Comparing Base APS, BatchGCP, and CF framework under Demographic Parity. For the CF framework, we vary $c\in\{0.05, 0.1, 0.15, 0.2\}$. In the figure, Base APS = Black lines, BatchGCP = Red lines, and the CF framework is the bar charts. The black dots are the \textit{desired} disparity level for the CF framework.}%, which the CF framework achieves, while neither Base APS nor BatchGCP meets these thresholds.}
    \label{fig:credit_dem_parity_gcp}
\end{figure}

\begin{figure}[ht!]
    \centering
    \begin{subfigure}{0.8\textwidth}
        \begin{subfigure}{0.5\textwidth}
            \includegraphics[width=\linewidth]{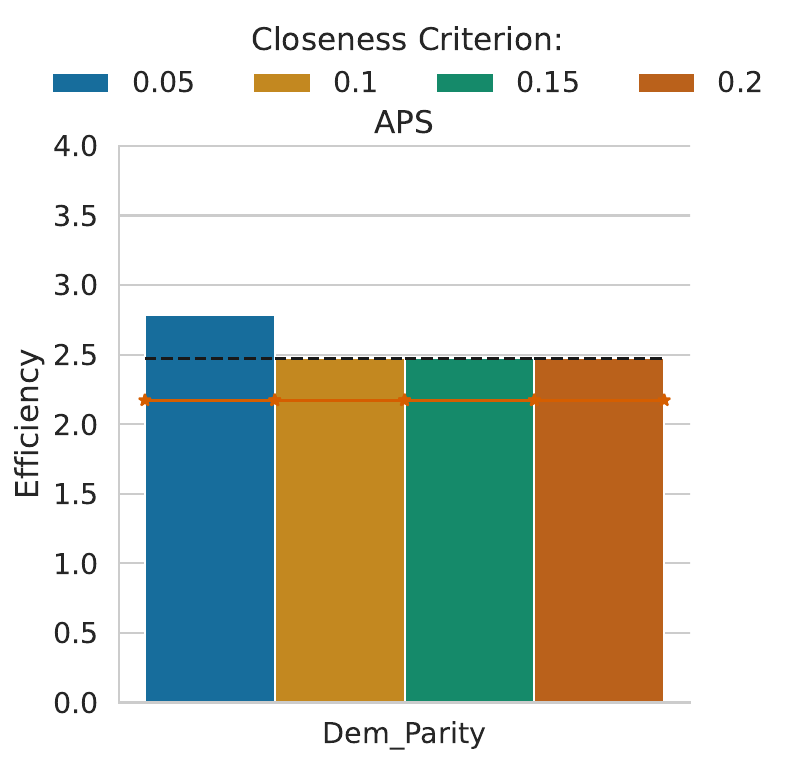}
        \end{subfigure}%
        \begin{subfigure}{0.5\textwidth}
            \includegraphics[width=\linewidth]{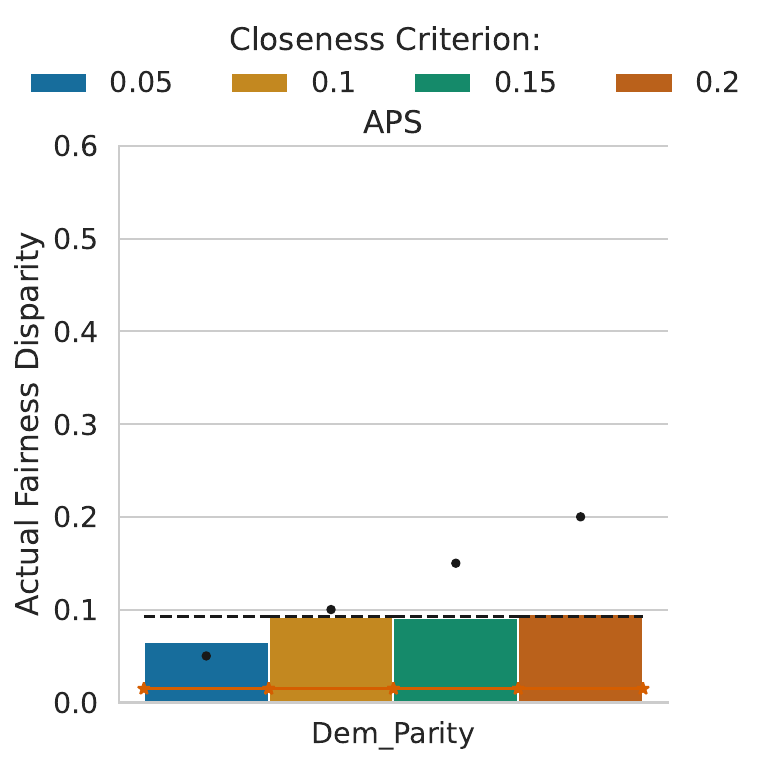}
        \end{subfigure}
        \caption{\small\textbf{Gender.}}
    \end{subfigure}
    \begin{subfigure}{0.8\textwidth}
        \begin{subfigure}{0.5\textwidth}
            \includegraphics[width=\linewidth]{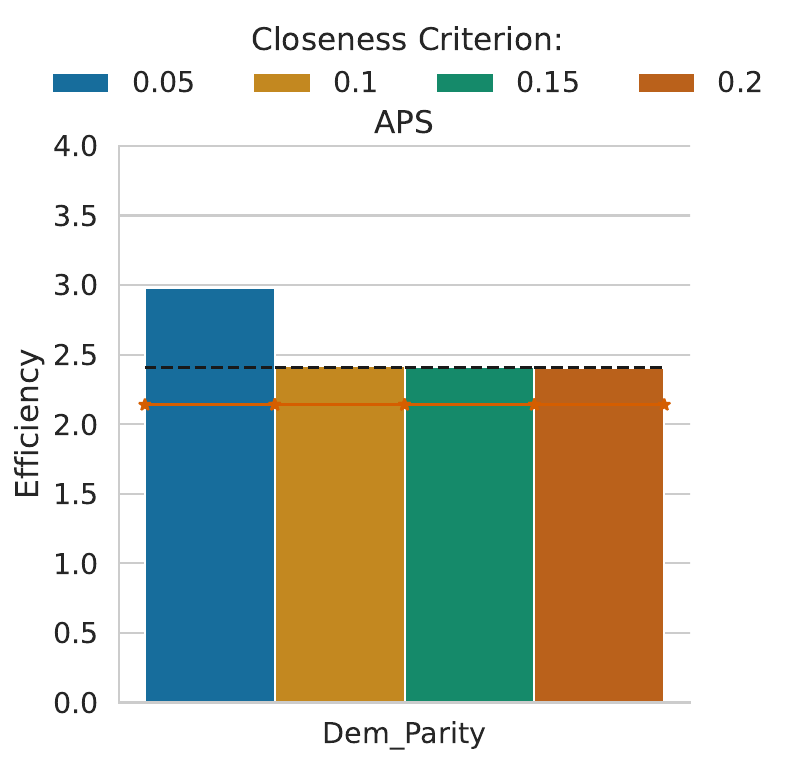}
        \end{subfigure}%
        \begin{subfigure}{0.5\textwidth}
            \includegraphics[width=\linewidth]{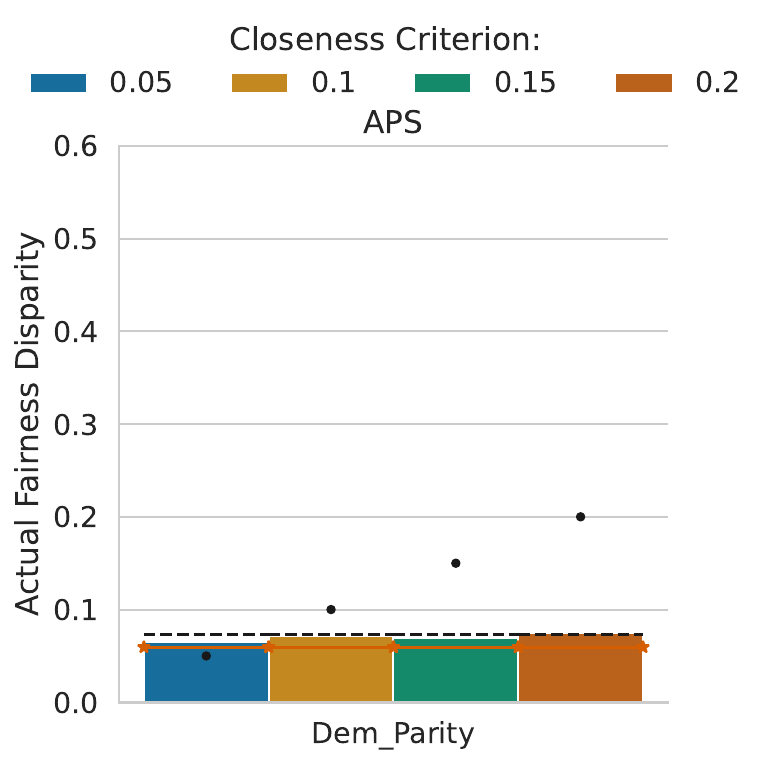}
        \end{subfigure}
        \caption{\small\textbf{Region.}}
    \end{subfigure}
    \begin{subfigure}{0.8\textwidth}
        \begin{subfigure}{0.5\textwidth}
            \includegraphics[width=\linewidth]{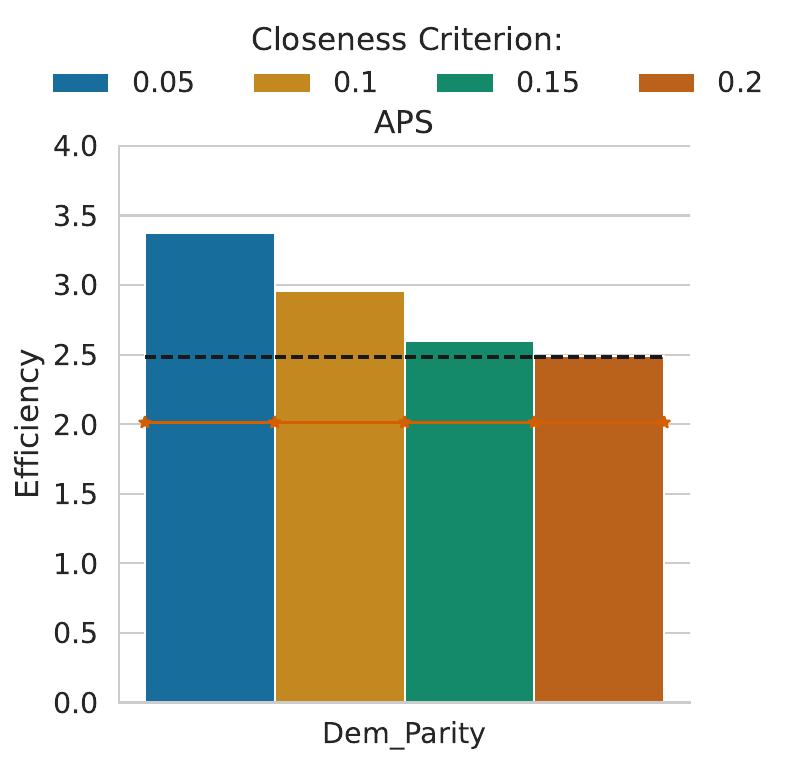}
        \end{subfigure}%
        \begin{subfigure}{0.5\textwidth}
            \includegraphics[width=\linewidth]{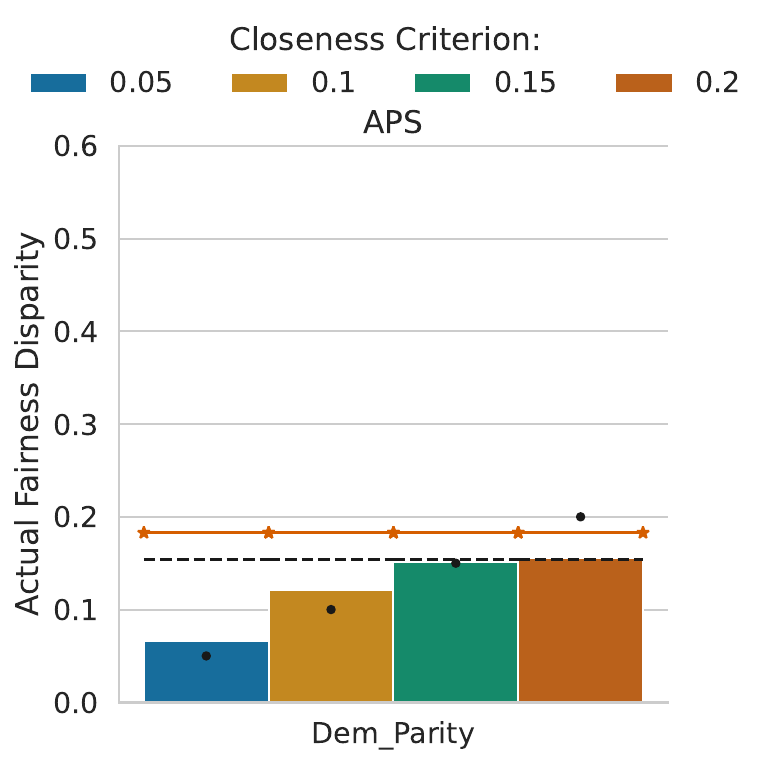}
        \end{subfigure}
        \caption{\small\textbf{Region \& Gender.}}
    \end{subfigure}
    \caption{\small\textbf{Pokec-n.} Comparing Base APS, BatchGCP, and CF framework under Demographic Parity. For the CF framework, we vary $c\in\{0.05, 0.1, 0.15, 0.2\}$. In the figure, Base APS = Black lines, BatchGCP = Red lines, and the CF framework is the bar charts. The black dots are the \textit{desired} disparity level for the CF framework.}%, which the CF framework achieves, while neither Base APS nor BatchGCP meets these thresholds.}
    \label{fig:pokec_n_dem_parity_gcp}
\end{figure}

\begin{figure}[ht!]
    \centering
    \begin{subfigure}{0.8\textwidth}
        \begin{subfigure}{0.5\textwidth}
            \includegraphics[width=\linewidth]{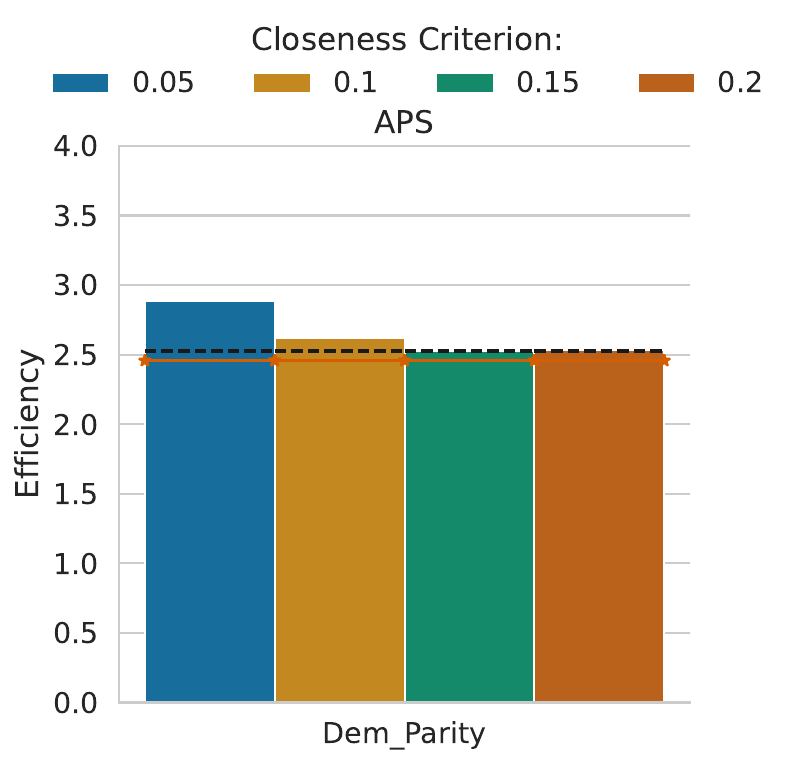}
        \end{subfigure}%
        \begin{subfigure}{0.5\textwidth}
            \includegraphics[width=\linewidth]{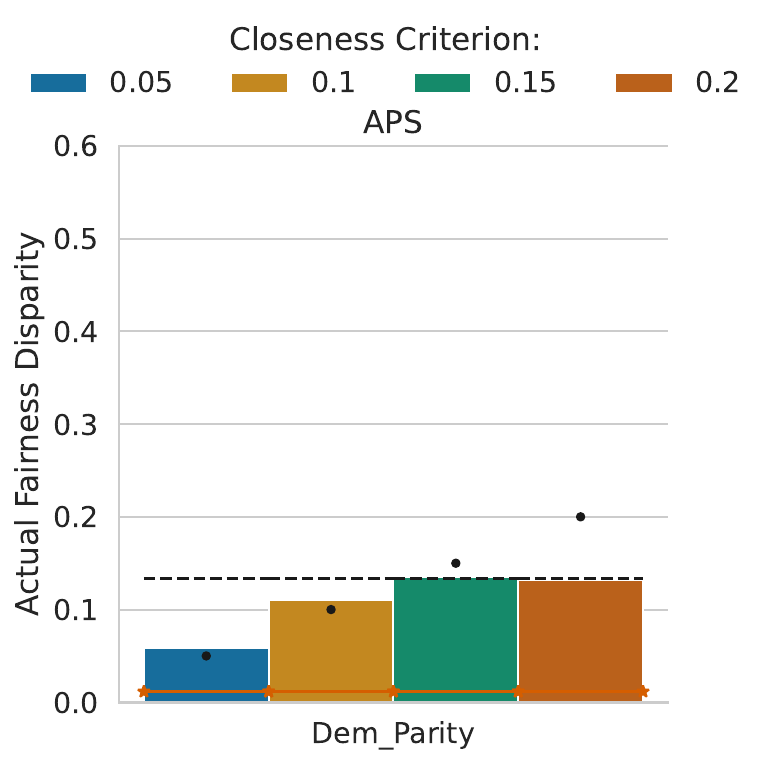}
        \end{subfigure}
        \caption{\small\textbf{Gender.}}
    \end{subfigure}
    \begin{subfigure}{0.8\textwidth}
        \begin{subfigure}{0.5\textwidth}
            \includegraphics[width=\linewidth]{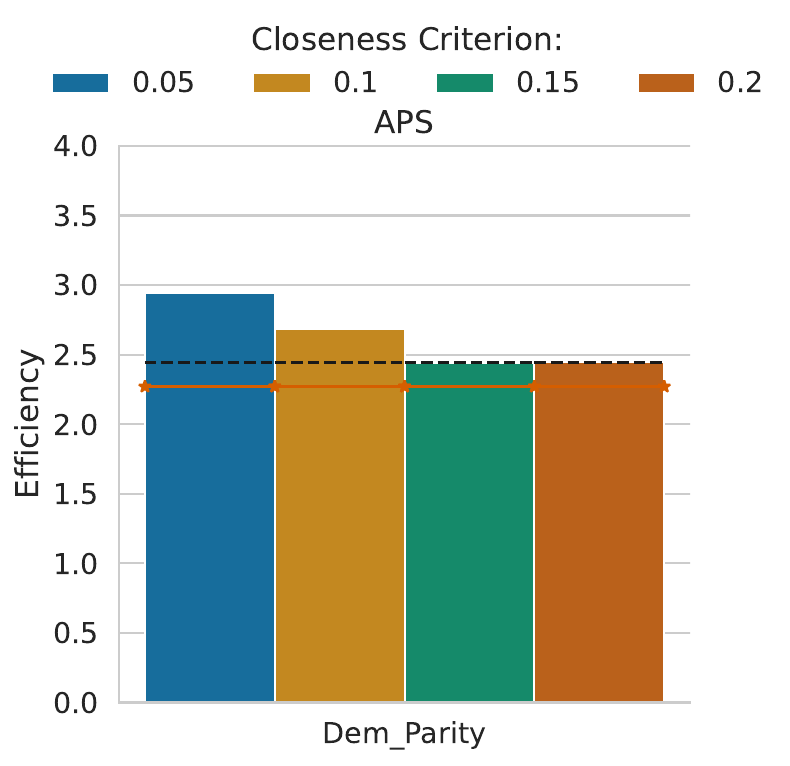}
        \end{subfigure}%
        \begin{subfigure}{0.5\textwidth}
            \includegraphics[width=\linewidth]{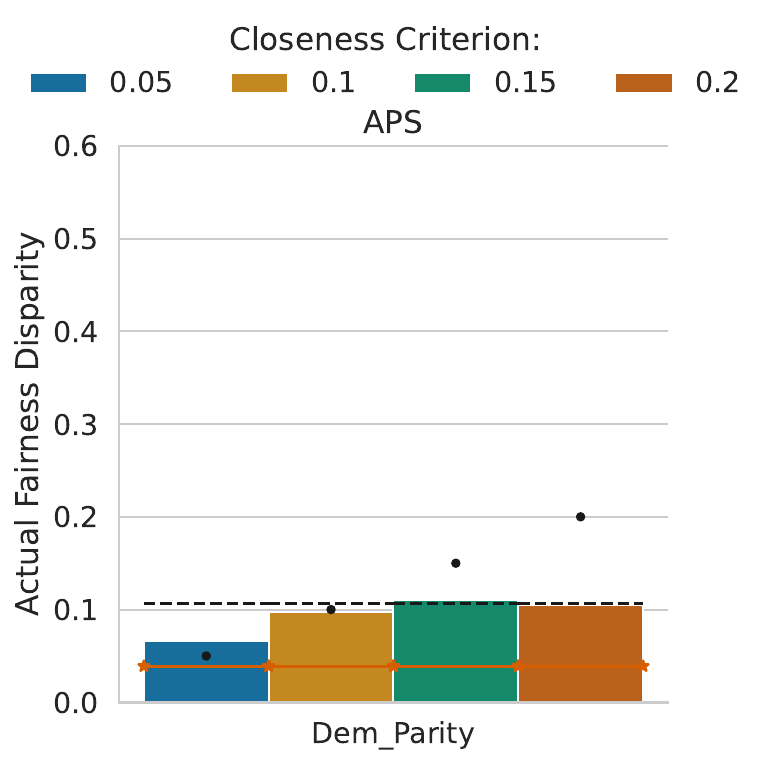}
        \end{subfigure}
        \caption{\small\textbf{Region.}}
    \end{subfigure}
    \begin{subfigure}{0.8\textwidth}
        \begin{subfigure}{0.5\textwidth}
            \includegraphics[width=\linewidth]{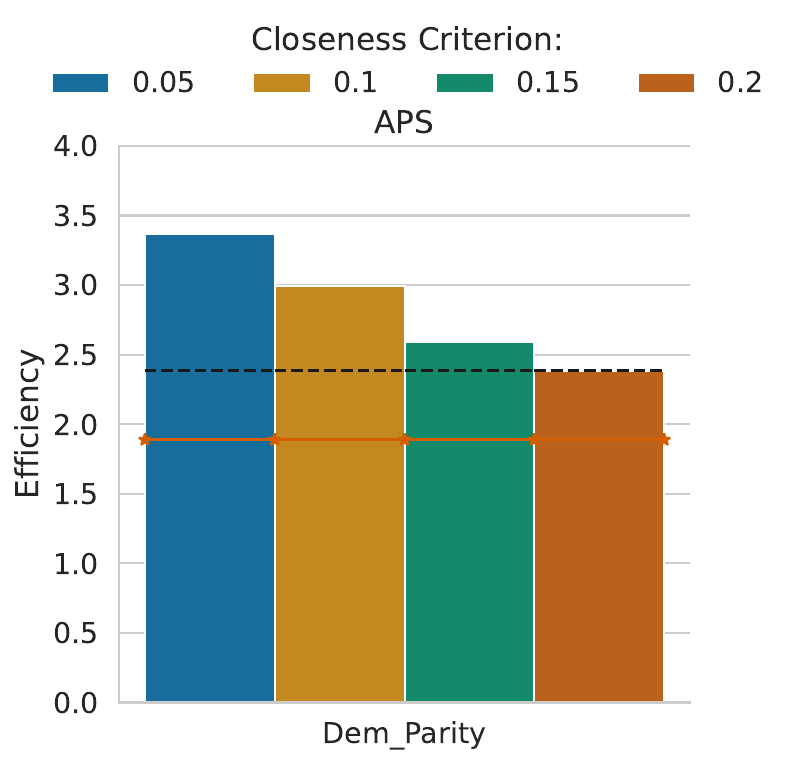}
        \end{subfigure}%
        \begin{subfigure}{0.5\textwidth}
            \includegraphics[width=\linewidth]{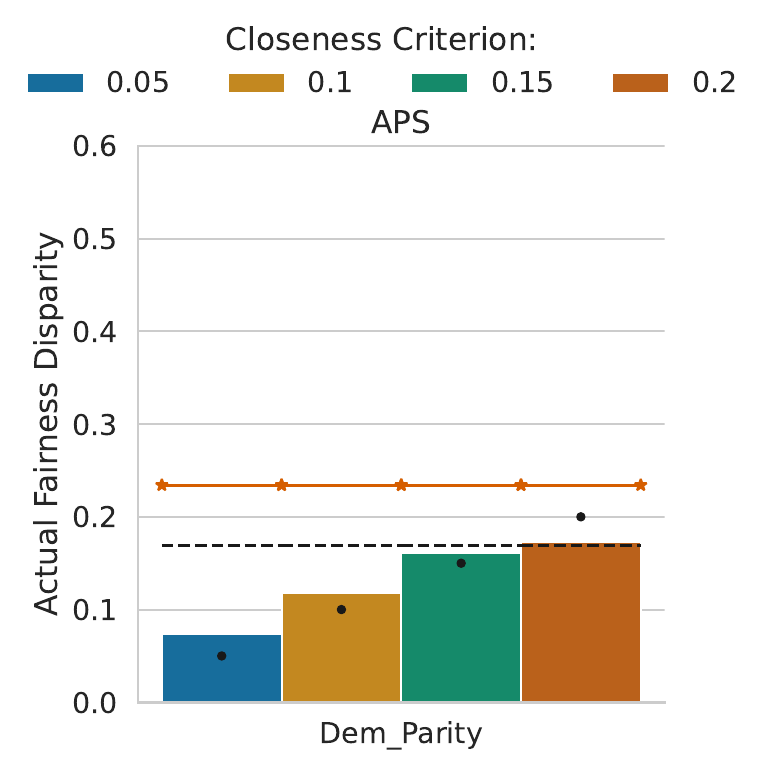}
        \end{subfigure}
        \caption{\small\textbf{Region \& Gender.}}
    \end{subfigure}
    \caption{\small\textbf{Pokec-z.} Comparing Base APS, BatchGCP, and CF framework under Demographic Parity. For the CF framework, we vary $c\in\{0.05, 0.1, 0.15, 0.2\}$. In the figure, Base APS = Black lines, BatchGCP = red lines, and the CF framework is the bar charts. The black dots are the \textit{desired} disparity level for the CF framework} %, which the CF framework achieves, while neither Base APS nor BatchGCP meets these thresholds.}
    \label{fig:pokec_z_dem_parity_gcp}
\end{figure}

\begin{figure}[ht!]
    \centering
    \begin{subfigure}{\textwidth}
        \begin{subfigure}{0.35\textwidth}
            \includegraphics[width=\linewidth]{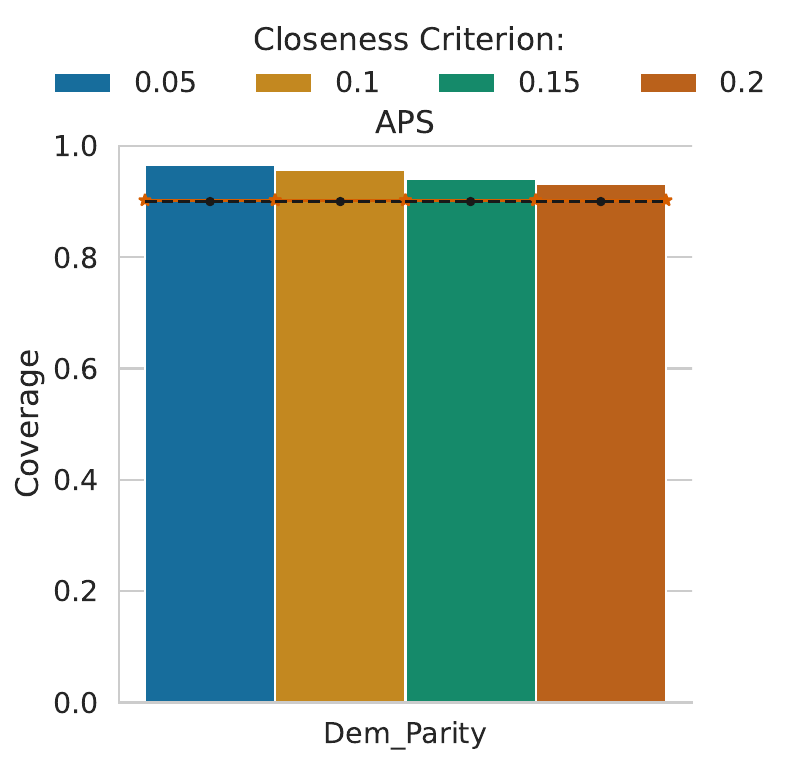}
            \caption{\small\textbf{ACSIncome.} }
        \end{subfigure}%
        \begin{subfigure}{0.35\textwidth}
            \includegraphics[width=\linewidth]{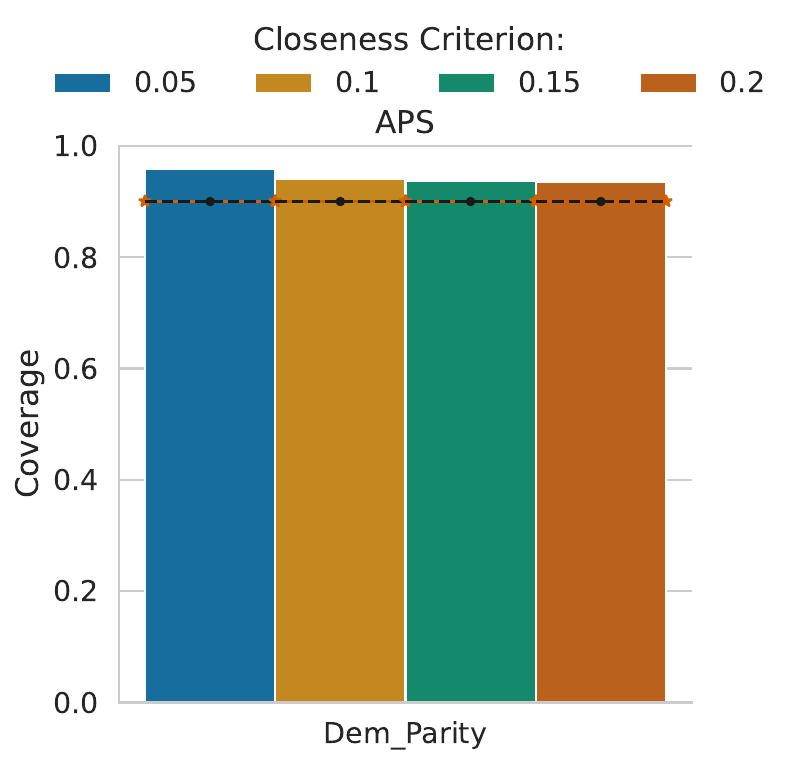}
            \caption{\small\textbf{ACSEducation.} }
        \end{subfigure}%
        \begin{subfigure}{0.35\textwidth}
            \includegraphics[width=\linewidth]{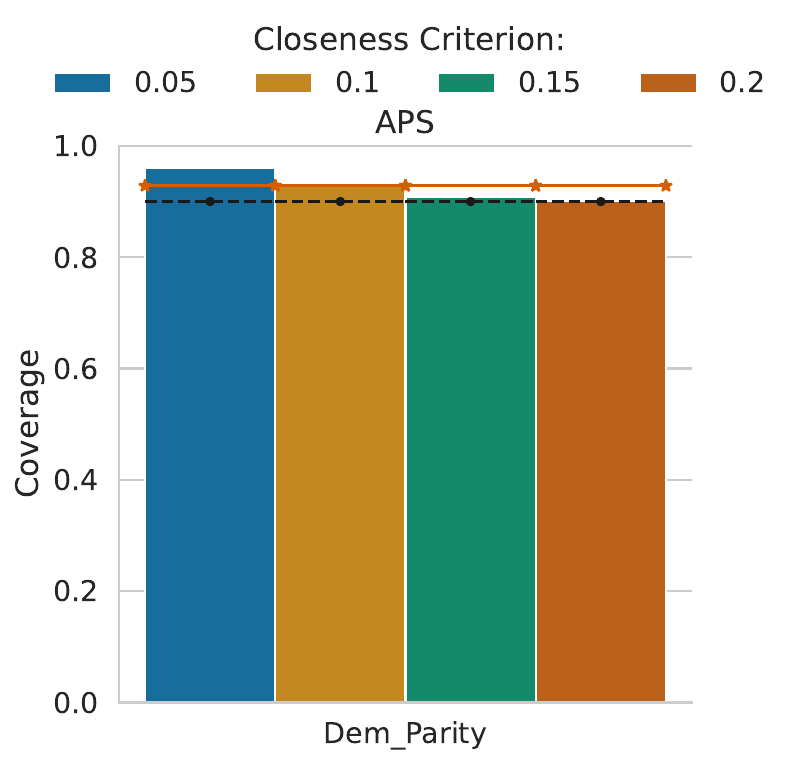}
            \caption{\small\textbf{Credit.} }
        \end{subfigure}
    \end{subfigure}

    \begin{subfigure}{\textwidth}
        \begin{subfigure}{0.35\textwidth}
            \includegraphics[width=\linewidth]{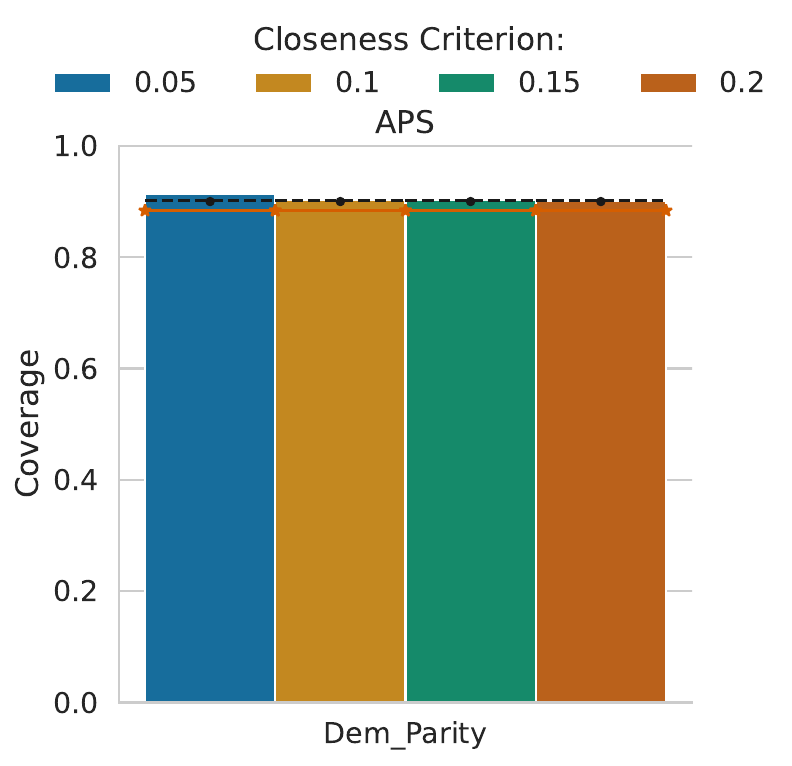}
            \caption{\small\textbf{Pokec-n, Gender.} }
        \end{subfigure}%
        \begin{subfigure}{0.35\textwidth}
            \includegraphics[width=\linewidth]{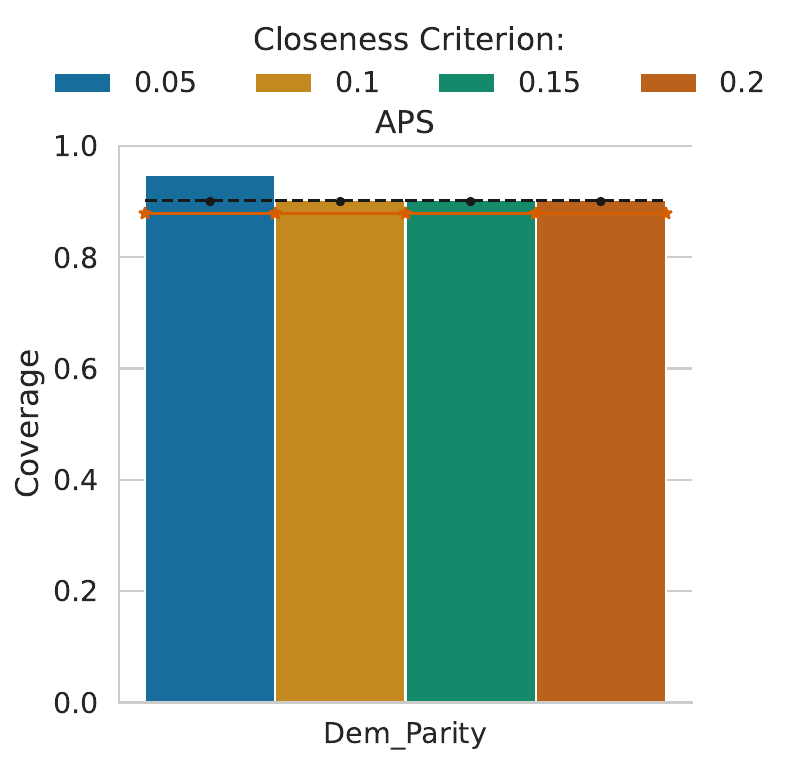}
            \caption{\small\textbf{Pokec-n, Region.} }
        \end{subfigure}%
        \begin{subfigure}{0.35\textwidth}
            \includegraphics[width=\linewidth]{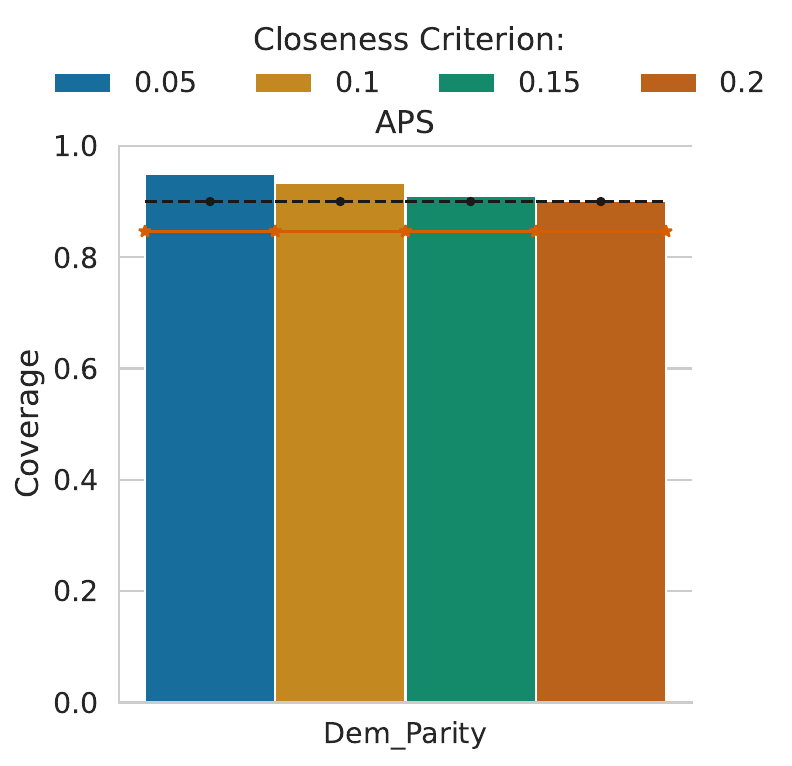}
            \caption{\small\textbf{Pokec-n, Region \& Gender.} }
        \end{subfigure}
    \end{subfigure}

    \begin{subfigure}{\textwidth}
        \begin{subfigure}{0.35\textwidth}
            \includegraphics[width=\linewidth]{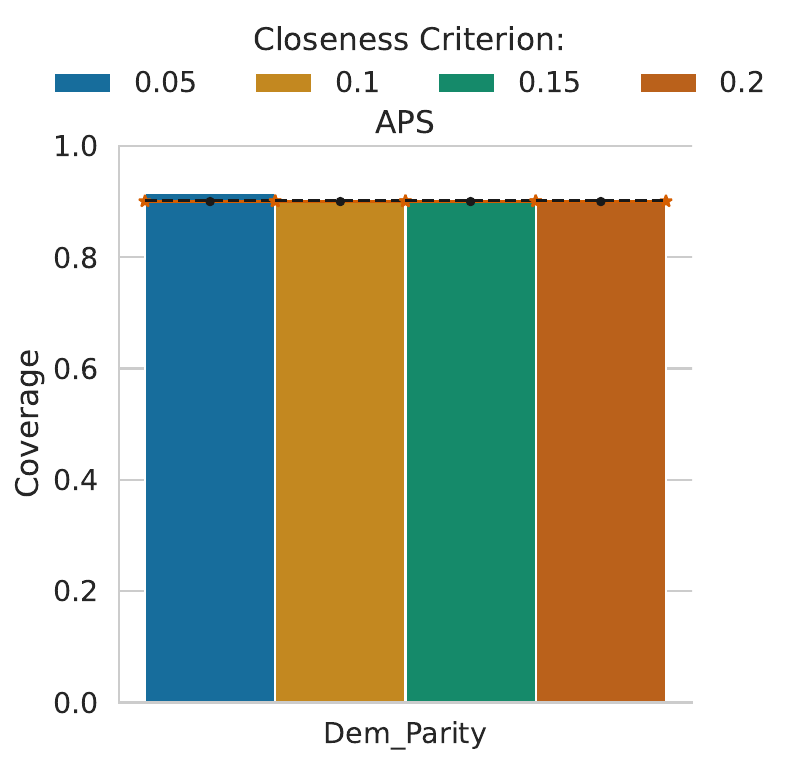}
            \caption{\small\textbf{Pokec-z, Gender.} }
        \end{subfigure}%
        \begin{subfigure}{0.35\textwidth}
            \includegraphics[width=\linewidth]{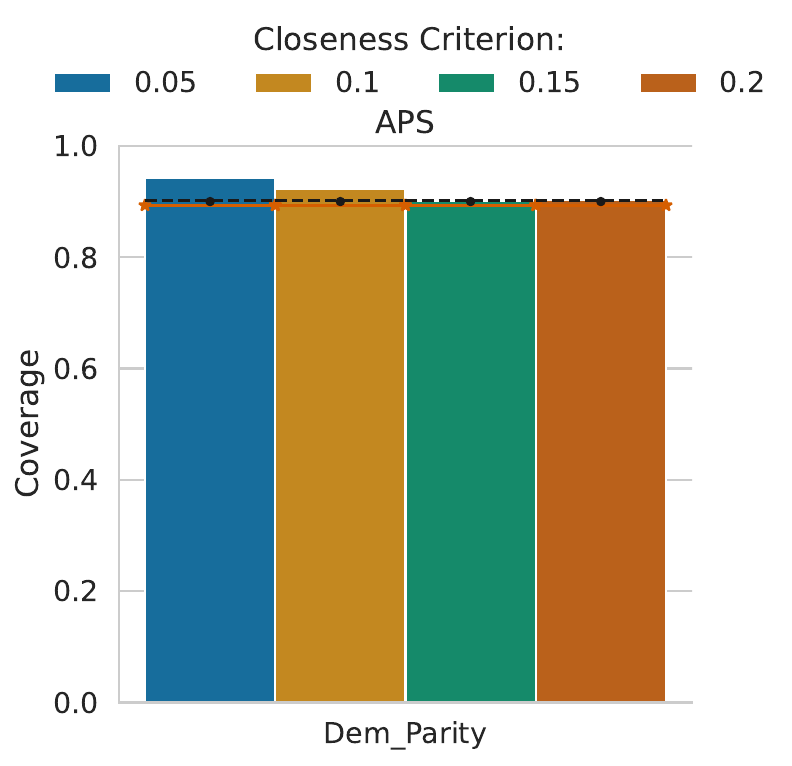}
            \caption{\small\textbf{Pokec-z, Region.} }
        \end{subfigure}%
        \begin{subfigure}{0.35\textwidth}
            \includegraphics[width=\linewidth]{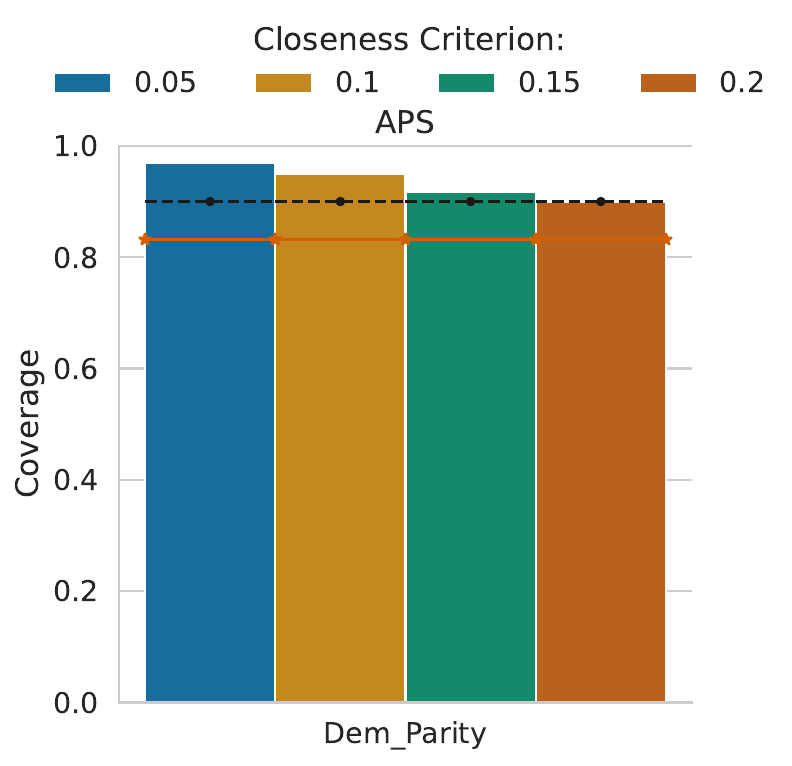}
            \caption{\small\textbf{Pokec-z, Region \& Gender.} }
        \end{subfigure}
    \end{subfigure}
    
    \caption{\small Comparing Overall Coverage of  Base APS, BatchGCP, and CF framework under Demographic Parity. For the CF framework, we vary $c\in\{0.05, 0.1, 0.15, 0.2\}$. In the figure, Base APS = Black lines, BatchGCP = Red lines, and the CF framework is the bar charts. The black dots are the \textit{desired} coverage level, which is $0.90$ for all methods.}
    \label{fig:all_coverages}
\end{figure}
